# Supplementary material for: Cooperative Self-Training for Multi-Target Adaptive Semantic Segmentation
Source: arXiv:2210.01578 source file (2022-10-04)
Supplement: Supplementary file 1 [file gamma.tex]

% This file was created with tikzplotlib v0.10.1.
\begin{tikzpicture}

\definecolor{darkslategray38}{RGB}{38,38,38}
\definecolor{lavender234234242}{RGB}{234,234,242}
\definecolor{lightgray204}{RGB}{204,204,204}
\definecolor{mediumseagreen85168104}{RGB}{85,168,104}
\definecolor{peru22113282}{RGB}{221,132,82}
\definecolor{steelblue76114176}{RGB}{76,114,176}

\begin{axis}[
axis background/.style={fill=lavender234234242},
axis line style={white},
height=0.5\textwidth,
legend cell align={left},
legend style={
  fill opacity=0.8,
  draw opacity=1,
  text opacity=1,
  at={(0.97,0.03)},
  anchor=south east,
  draw=lightgray204,
  fill=lavender234234242
},
tick align=outside,
width=0.6\textwidth,
x grid style={white},
xmajorgrids,
xmajorticks=false,
xmin=-4.9505579499372, xmax=2.64797285694315,
xtick style={color=darkslategray38},
y grid style={white},
ymajorgrids,
ymajorticks=false,
ymin=60, ymax=75,
ytick style={color=darkslategray38}
]
\addplot [semithick, steelblue76114176]
table {%
-4.60517018598809 71.1
-2.30258509299405 71.6
-1.6094379124341 70.9
-0.693147180559945 71.8
0 72.6
0.693147180559945 71.1
1.6094379124341 71.1
2.30258509299405 71.3
};
\addlegendentry{Cityscapes}
\addplot [semithick, peru22113282]
table {%
-4.60517018598809 69.9
-2.30258509299405 70
-1.6094379124341 70.1
-0.693147180559945 69.8
0 70
0.693147180559945 70.1
1.6094379124341 70.2
2.30258509299405 70
};
\addlegendentry{IDD}
\addplot [semithick, mediumseagreen85168104, dashed]
table {%
-4.60517018598809 70.5
-2.30258509299405 70.8
-1.6094379124341 70.5
-0.693147180559945 70.8
0 71.3
0.693147180559945 70.6
1.6094379124341 70.6
2.30258509299405 70.7
};
\addlegendentry{Avg}
\end{axis}

\end{tikzpicture}
